# Supplementary material for: MECHBench: A Set of Black-Box Optimization Benchmarks originated from Structural Mechanics
Source: arXiv:2511.10821 source file (2025-11-13)

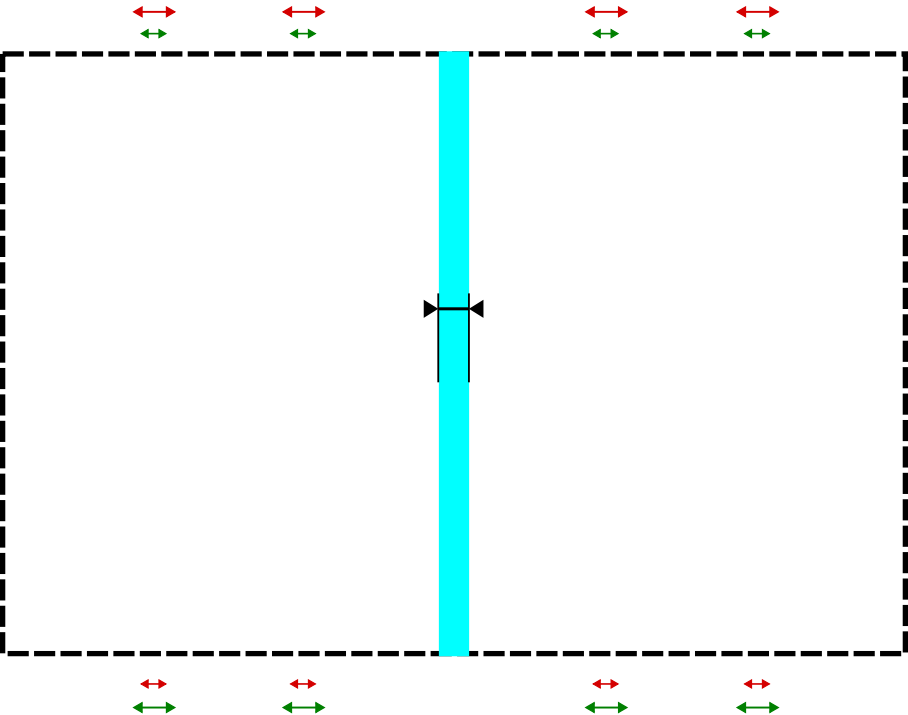

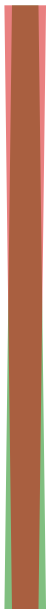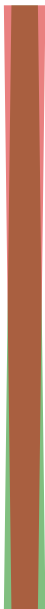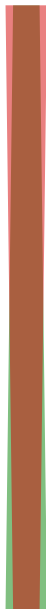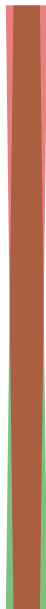

Supplement: Supplementary file 4 [file general_interpretation_sm2_5_svg-tex.pdf]
