# Supplementary material for: MECHBench: A Set of Black-Box Optimization Benchmarks originated from Structural Mechanics
Source: arXiv:2511.10821 source file (2025-11-13)

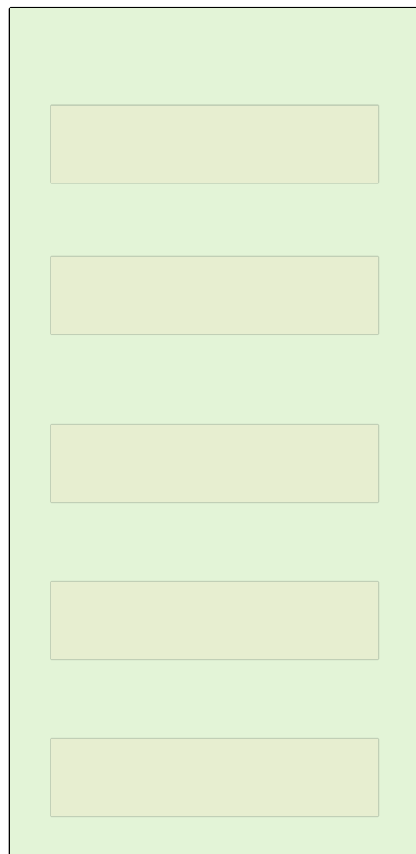

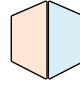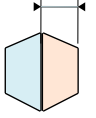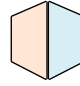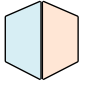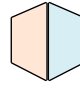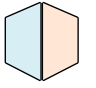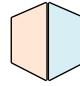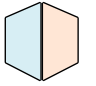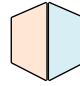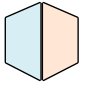

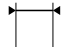

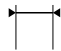

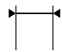

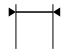

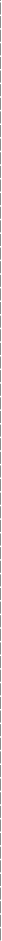

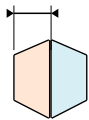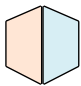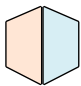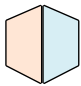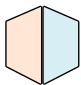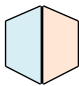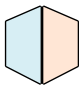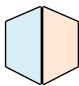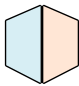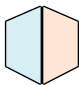



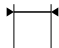

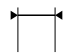

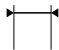

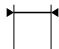

Supplement: Supplementary file 6 [file sm3_epsilon_edited_svg-tex.pdf]
